# Supplementary material for: Uncovering the nature of low-lying dipole states with QRPA calculations: is Z=42 the answer?
Source: arXiv:2507.23244 ancillary file (2025-07-31)
Supplement: Supplementary file 1 [file QRPA4NRT_PDR_v14-Suppl-sub.pdf]

# Supplementary Material: Uncovering the nature of low-lying dipole states with QRPA calculations: is Z=42 the answer?

E. J. In[1],* E. V. Chimanski[2], J. E. Escher [1], S. Péru[3], A. Thapa[1], and W. Younes[1]

*Lawrence Livermore National Laboratory, Livermore, 94550, CA, USA* [1]
*National Nuclear Data Center, Brookhaven National Laboratory, Upton, 11973, NY, USA* [2]
*CEA, DAM, DIF, Arpajon, France* [3]
*Université Paris-Saclay, CEA, LMCE, 91680 Bruyères-le-Châtel, France* [4]

(Dated: July 30, 2025)

This supplementary document provides additional results and detailed data to support the analysis presented in the main text of the paper (E. J. In *et al.*, main paper). In particular, it includes: (i) radial transition densities for $^{82-98}$Mo isotopes, including the states identified as skin oscillation candidates, the major PDR peak, and the major GDR peak in each isotope (see Sec. III C of the main paper), and (ii) tables summarizing the microscopic two-quasiparticle (2qp) configurations and collectivity indices of selected low-lying dipole states in $^{82-98}$Mo isotopes. The notation and classification criteria used in this document follow those defined in the main text.

## I. RADIAL TRANSITION DENSITIES FOR OTHER RELEVANT STATES

To investigate the spatial structure and isospin character of dipole excitations, we analyze the radial transition densities of dipole states in the low-energy enhanced dipole region, as exemplified in Fig. 3 of the main text. For each isotope, several skin oscillation states are presented, followed by the transition densities of the major PDR peak and the GDR peak. The figures are grouped and labeled by isotope, with the last two panels for each isotope corresponding to the major PDR and GDR peak, respectively.

These plots reveal a distinct pattern of skin oscillation states from major PDR and GDR peaks: in-phase oscillations of protons and neutrons in the nuclear interior, with dominant neutron or proton oscillations in the surface and beyond region, supporting the mixed isoscalar-isovector character discussed in the main text.

## II. MICROSCOPIC TWO-QUASIPARTICLE STRUCTURE OF LOW-LYING DIPOLE STATES

Table I and Table II summarize the microscopic structures of the identified dipole states for $^{82-90}$Mo and $^{92-98}$Mo, respectively. The skin oscillation states, the major PDR peaks (marked with $^{\dagger}$), and the major GDR peaks (marked with $^{*}$) are included. For each state, the QRPA excitation energy and fragmentation index are provided. Only two-quasiparticle (2qp) configurations contributing more than 10 % are listed.

The major GDR peaks in these isotopes exhibit the expected strong collectivity, characterized by a coherent superposition of numerous 2qp configurations. In contrast, the skin oscillation states, particularly in nuclei with a proton skin, display varying fragmentation numbers. In $^{82}$Mo and $^{84}$Mo, for example, skin oscillation states at $E$ =16.03 and 16.63 MeV are dominated by the single proton 2qp configuration, $(1g_{9/2}, 2f_{7/2})_\pi$, with significant proton contributions of 92 % and 86 %, respectively. This dominant configuration involves weakly bound proton orbitals near the Fermi surface. These states exhibit low fragmentation indices, with relative $R$ values of 0.44 and 0.54, respectively, reflecting their single-particle-like nature.

Note that $^{94}$Mo, $^{96}$Mo, and $^{98}$Mo exhibit skin oscillation behavior near 10 and 11 MeV similar to $^{90}$Mo. For example, the states at $E$ = 10.28 MeV in $^{94}$Mo and 10.36 MeV in $^{96}$Mo have nearly equal neutron and proton contributions. These states are dominated by $(2p_{1/2}, 3s_{1/2})_{\pi,\nu}$ configurations, similar to the $E = 10.17$ MeV state in $^{90}$Mo. In contrast, the states at $E = 11.24$ MeV in $^{90}$Mo and $E = 11.31$ MeV in $^{94}$Mo are mainly generated by $(2p_{1/2}, 2d_{3/2})_\pi$ and $(2p_{3/2}, 2d_{5/2})_\pi$ configurations. Additionally, the $E = 11.24$ MeV state in $^{94}$Mo, and the $E = 11.33$ MeV states in $^{96}$Mo and $^{98}$Mo are primarily generated by the $(2d_{5/2}, 2f_{7/2})_\nu$ configuration. Notably, the $E = 11.33$ MeV states exhibit slightly stronger proton contributions, similar to the $E = 11.24$ MeV state in $^{90}$Mo.

In addition, skin oscillation states near 12.5 MeV and 14.5 MeV are observed exclusively in nuclei with a neutron skin. States near 14 MeV are mainly generated by proton configurations such as $(1f_{5/2}, 2d_{3/2})_\pi$ and $(2p_{3/2}, 2d_{3/2})_\pi$, while those near 12.5 MeV involve strongly neutron-dominated configurations such as $(1g_{7/2}, 2f_{7/2})_\nu$, $(1f_{5/2}, 2d_{5/2})_\nu$ and $(2d_{5/2}, 3p_{3/2})_\nu$.

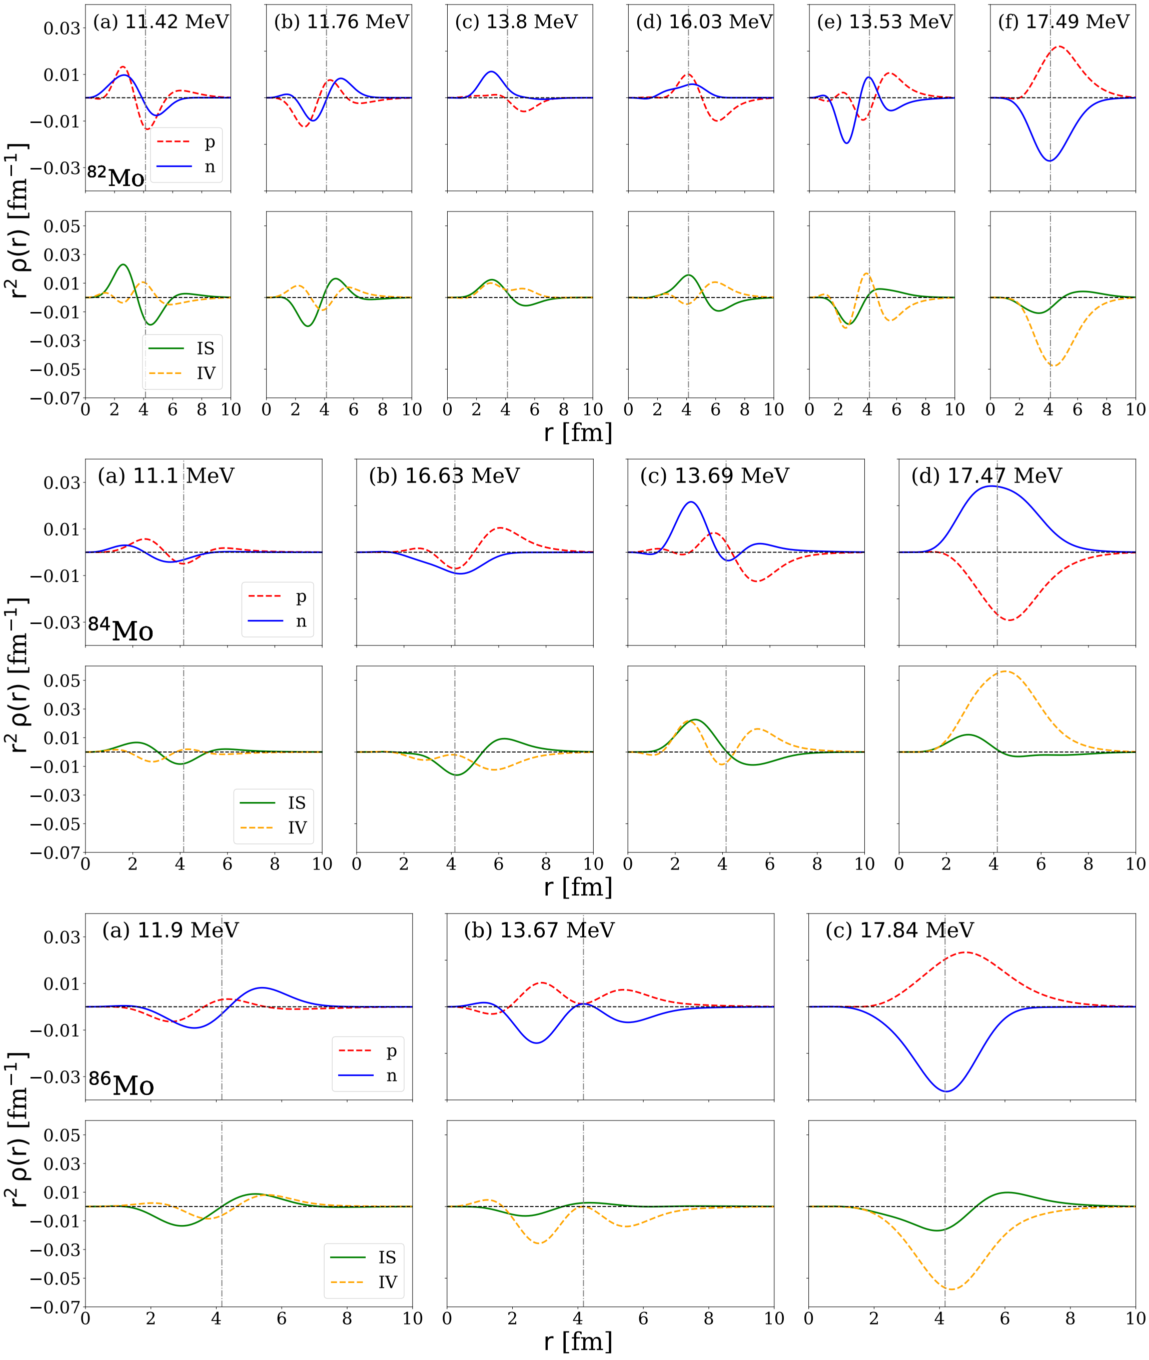


FIG. 1: Radial transition densities for dipole states in $^{82,84,86}$Mo isotopes, including skin oscillation states, the major PDR peak, and the major GDR peak. In each panel, the upper subfigure displays proton (red dashed) and neutron (blue solid) transition densities, with the vertical gray dashed lines indicating the ground-state rms radii from HFB calculations. The lower subfigure presents the corresponding $IS$ (green solid) and $IV$ (yellow dashed) transition densities. The last two columns (panels (e) and (f) for $^{82}$Mo, (c) and (d) for $^{84}$Mo, and (b) and (c) for $^{86}$Mo) correspond to the major PDR and GDR peaks, respectively, highlighting the distinct features between low-energy and giant dipole states.

* in2@llnl.gov

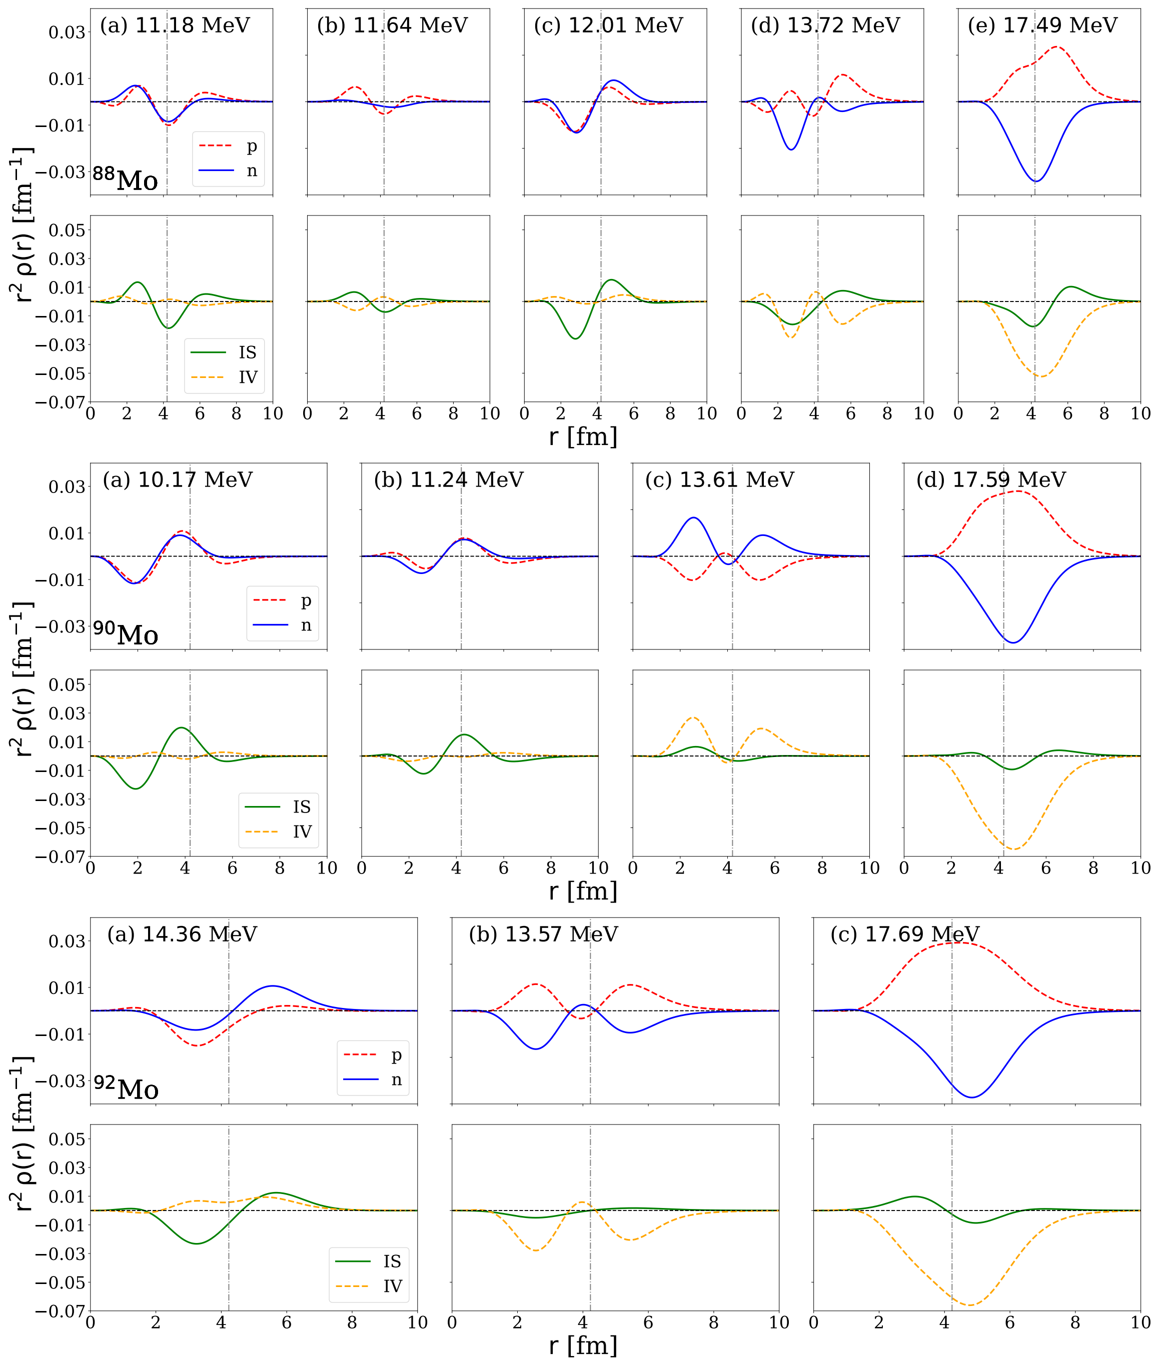


FIG. 2: Same as Fig 1, but for $^{88,90,92}$Mo isotopes.

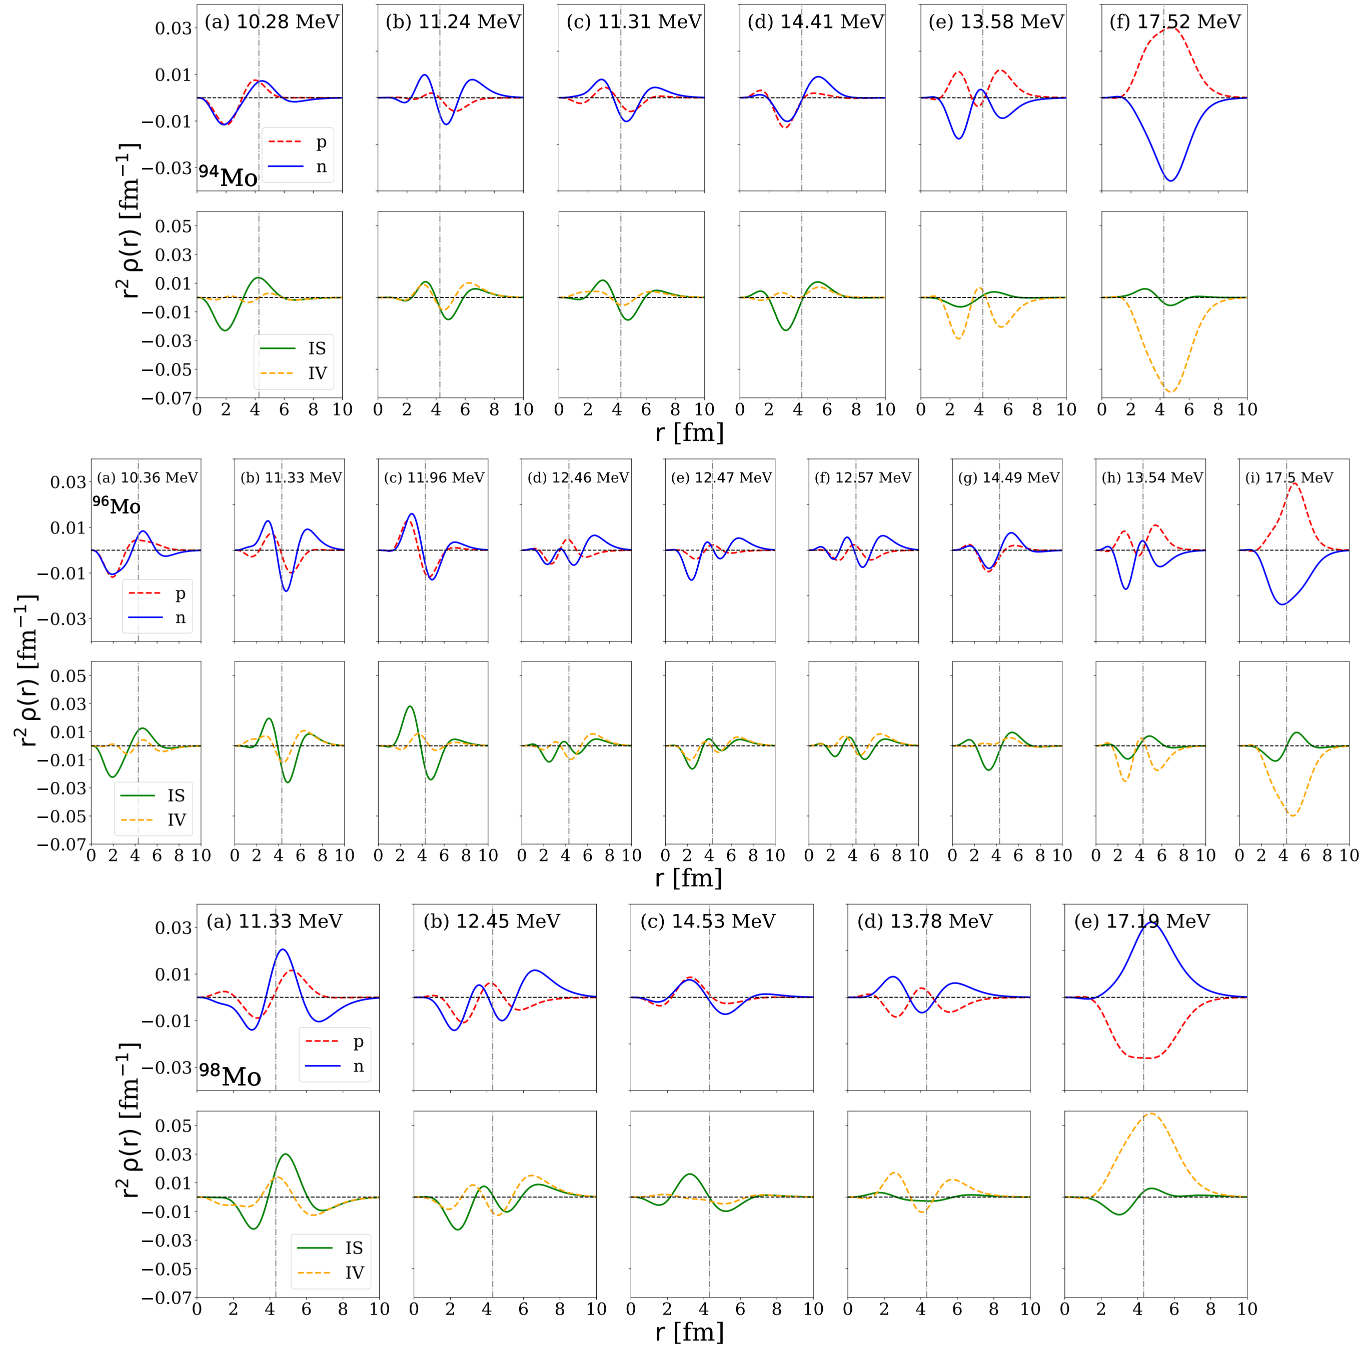


FIG. 3: Same as Fig 1, but for $^{94,96,98}$Mo isotopes.

TABLE I: QRPA excited state energies (in MeV), main two-quasiparticle configurations, and collectivity indexes for the low-lying dipole excitations, the major peak of the PDR region (denoted by $^{\dagger}$) and the major GDR peak (denoted by $^{*}$) in $^{82-90}$Mo isotopes. The columns include excitation energies ($w$), dominant 2qp configurations with their contributions (in percentage), the total number of contributing 2qp configurations ($N^{*}$), the number of contributing 2qp configurations from neutrons ($N^{*}_{\nu}$) and protons ($N^{*}_{\pi}$), the relative fragmentation ratio ($R$), and the percentage contributions of neutron (%($\nu$)) and proton (%($\pi$)) components.

| Isotopes | $w$ [MeV] | Structure %[2qp pair]$_{q=\nu,\pi}$ | $N^{*}$ | $N^{*}_{\nu}$ | $N^{*}_{\pi}$ | $R$ | % ($\nu$) | % ($\pi$) |
|---|---|---|---|---|---|---|---|---|
| $^{82}$Mo | 11.42 | $59.7[1f_{5/2}2d_{5/2}]_{\nu} + 12.9[2p_{3/2}2d_{5/2}]_{\pi}$ | 110 | 44 | 66 | 0.61 | 68.1 | 32.0 |
| $^{82}$Mo | 11.76 | $34.6[1g_{9/2}1h_{11/2}]_{\pi} + 11.4[2p_{1/2}2d_{3/2}]_{\pi} + 11.0[1f_{5/2}1g_{7/2}]_{\pi}$ | 130 | 52 | 78 | 0.72 | 27.0 | 73.0 |
| $^{82}$Mo | 13.80 | $69.4[1g_{9/2}1h_{11/2}]_{\nu} + 13.2[1f_{5/2}2d_{3/2}]_{\nu}$ | 148 | 90 | 58 | 0.82 | 92.8 | 7.2 |
| $^{82}$Mo | 16.03 | $92.1[1g_{9/2}2f_{7/2}]_{\pi}$ | 80 | 32 | 48 | 0.44 | 2.2 | 97.8 |
| $^{82}$Mo | 13.53$^{\dagger}$ | $20.5[2p_{3/2}2d_{5/2}]_{\nu} + 15.9[1f_{5/2}1g_{7/2}]_{\pi} + 13.4[1h_{11/2}1g_{9/2}]_{\nu} + 11.9[1f_{5/2}2d_{3/2}]_{\pi}$ | 126 | 74 | 52 | 0.70 | 64.6 | 35.4 |
| $^{82}$Mo | 17.49$^{*}$ | $29.3[1f_{7/2}2d_{5/2}]_{\nu} + 24.5[1d_{3/2}2p_{1/2}]_{\nu} + 13.4[1f_{5/2}1g_{7/2}]_{\nu}$ | 180 | 84 | 96 | | 83.1 | 16.9 |
| $^{84}$Mo | 11.10 | $48.1[1f_{5/2}2d_{5/2}]_{\pi} + 18.6[2p_{3/2}2d_{5/2}]_{\pi} + 13.0[2p_{1/2}2d_{3/2}]_{\pi}$ | 58 | 26 | 32 | 0.32 | 10.3 | 89.7 |
| $^{84}$Mo | 16.63 | $86.3[1g_{9/2}2f_{7/2}]_{\pi} + 10.5[1f_{7/2}2d_{5/2}]_{\pi}$ | 98 | 40 | 58 | 0.54 | 1.7 | 98.3 |
| $^{84}$Mo | 13.69$^{\dagger}$ | $22.5[1f_{5/2}2d_{3/2}]_{\nu} + 15.9[1f_{5/2}1g_{7/2}]_{\pi} + 15.4[2p_{3/2}2d_{5/2}]_{\nu} + 13.0[2p_{3/2}2d_{3/2}]_{\nu}$ | 138 | 70 | 68 | 0.77 | 68.6 | 31.4 |
| $^{84}$Mo | 17.47$^{*}$ | $35.1[1f_{7/2}2d_{5/2}]_{\nu} + 18.1[1f_{5/2}1g_{7/2}]_{\nu}$ | 180 | 84 | 96 | | 73.0 | 27.0 |
| $^{86}$Mo | 11.90 | $47.6[1f_{7/2}1g_{9/2}]_{\nu} + 30.0[1g_{9/2}1h_{11/2}]_{\nu}$ | 146 | 92 | 54 | 0.87 | 85.0 | 15.0 |
| $^{86}$Mo | 13.67$^{\dagger}$ | $20.1[1f_{5/2}2d_{3/2}]_{\pi} + 15.7[1f_{5/2}1g_{7/2}]_{\nu}$ | 138 | 64 | 74 | 0.82 | 51.5 | 48.5 |
| $^{86}$Mo | 17.84$^{*}$ | $51.9[1g_{9/2}2f_{7/2}]_{\nu} + 11.0[1f_{5/2}1g_{7/2}]_{\nu}$ | 168 | 80 | 88 | | 75.9 | 24.1 |
| $^{88}$Mo | 11.18 | $38.3[2p_{1/2}2d_{3/2}]_{\pi} + 11.0[2p_{3/2}2d_{5/2}]_{\pi}$ | 98 | 56 | 42 | 0.72 | 28.3 | 71.7 |
| $^{88}$Mo | 11.64 | $63.2[1f_{5/2}2d_{5/2}]_{\pi} + 10.3[2p_{3/2}2d_{5/2}]_{\pi}$ | 90 | 40 | 50 | 0.66 | 5.3 | 94.7 |
| $^{88}$Mo | 12.01 | $25.8[1g_{9/2}1h_{11/2}]_{\pi} + 20.9[1f_{5/2}1g_{7/2}]_{\pi} + 14.6[2p_{1/2}2d_{3/2}]_{\pi} + 10.4[1f_{5/2}1g_{7/2}]_{\nu}$ | 148 | 76 | 72 | 1.09 | 30.7 | 69.3 |
| $^{88}$Mo | 13.72$^{\dagger}$ | $21.1[1f_{5/2}2d_{3/2}]_{\nu} + 17.0[3s_{1/2}2p_{3/2}]_{\pi} + 11.5[1f_{5/2}1g_{7/2}]_{\pi} + 11.4[2p_{3/2}2d_{3/2}]_{\nu}$ | 128 | 66 | 62 | 0.94 | 51.1 | 48.9 |
| $^{88}$Mo | 17.49$^{*}$ | $24.1[1g_{9/2}2f_{7/2}]_{\pi} + 14.5[1f_{7/2}2d_{5/2}]_{\pi} + 13.7[1f_{5/2}1g_{7/2}]_{\nu}$ | 136 | 72 | 64 | | 56.1 | 44.0 |
| $^{90}$Mo | 10.17 | $27.9[2p_{1/2}3s_{1/2}]_{\nu} + 25.4[2p_{1/2}3s_{1/2}]_{\pi} + 19.7[2p_{3/2}2d_{5/2}]_{\pi} + 15.6[2p_{3/2}2d_{5/2}]_{\nu}$ | 114 | 56 | 58 | 0.66 | 49.3 | 50.7 |
| $^{90}$Mo | 11.24 | $29.5[2p_{1/2}2d_{3/2}]_{\pi} + 11.8[2p_{3/2}2d_{5/2}]_{\pi} + 10.5[2p_{1/2}2d_{3/2}]_{\nu}$ | 110 | 58 | 52 | 0.63 | 36.3 | 63.7 |
| $^{90}$Mo | 13.61$^{\dagger}$ | $16.5[2d_{3/2}2p_{3/2}]_{\pi} + 15.1[1f_{5/2}1g_{7/2}]_{\nu} + 12.9[1f_{5/2}1g_{7/2}]_{\pi} + 10.1[2p_{3/2}2d_{5/2}]_{\nu}$ | 128 | 66 | 62 | 0.74 | 51.1 | 48.9 |
| $^{90}$Mo | 17.59$^{*}$ | $23.8[1f_{7/2}2d_{5/2}]_{\pi} + 17.3[1f_{5/2}1g_{7/2}]_{\pi} + 11.8[1f_{5/2}1g_{7/2}]_{\nu} + 10.3[1f_{7/2}1g_{9/2}]_{\pi}$ | 174 | 78 | 96 | | 33.3 | 66.7 |

TABLE II: Same as Table I, but for $^{92-98}$Mo isotopes.

| Isotopes | $w$ (MeV) | Structure %[2qp pair]$_{q=\nu,\pi}$ | $N^*$ | $N^*_\nu$ | $N^*_\pi$ | $R$ | % ($\nu$) | % ($\pi$) |
|---|---|---|---|---|---|---|---|---|
| $^{92}$Mo | 14.36 | $37.2[1f_{5/2}2d_{3/2}]_\pi + 22.5[2p_{3/2}2d_{3/2}]_\pi$ | 124 | 56 | 68 | 0.69 | 27.2 | 72.8 |
| $^{92}$Mo | 13.57$^\dagger$ | $18.3[1f_{5/2}1g_{7/2}]_\pi + 12.9[2p_{3/2}2d_{3/2}]_\pi +$ $11.2[2p_{3/2}2d_{5/2}]_\nu + 10.5[1f_{5/2}1g_{7/2}]_\nu + 10.2[1f_{5/2}2d_{3/2}]_\nu$ | 112 | 62 | 50 | 0.62 | 51.3 | 48.7 |
| $^{92}$Mo | 17.69$^*$ | $29.0[1f_{7/2}2d_{5/2}]_\pi + 21.4[1f_{5/2}1g_{7/2}]_\pi + 10.4[1g_{9/2}1h_{11/2}]_\nu$ | 180 | 78 | 102 | | 23.7 | 76.3 |
| $^{94}$Mo | 10.28 | $34.1[2p_{1/2}3s_{1/2}]_\nu + 28.0[2p_{1/2}3s_{1/2}]_\pi + 15.8[2p_{3/2}2d_{5/2}]_\pi$ | 120 | 66 | 54 | 0.63 | 53.0 | 47.0 |
| $^{94}$Mo | 11.24 | $65.7[2d_{5/2}2f_{7/2}]_\nu + 11.1[2d_{5/2}3p_{3/2}]_\nu$ | 164 | 114 | 50 | 0.86 | 88.4 | 11.6 |
| $^{94}$Mo | 11.31 | $21.4[2p_{3/2}2d_{5/2}]_\pi + 19.5[2p_{1/2}2d_{3/2}]_\pi + 14.3[1f_{5/2}2d_{5/2}]_\pi$ | 154 | 102 | 52 | 0.81 | 36.6 | 63.4 |
| $^{94}$Mo | 14.41 | $25.7[1f_{5/2}2d_{3/2}]_\pi + 24.1[2p_{3/2}2d_{3/2}]_\pi + 13.7[2p_{3/2}3s_{1/2}]_\pi + 10.6[1f_{5/2}2d_{3/2}]_\nu$ | 116 | 76 | 40 | 0.61 | 29.4 | 70.6 |
| $^{94}$Mo | 13.58$^\dagger$ | $17.4[1f_{5/2}1g_{7/2}]_\pi + 12.9[1f_{5/2}1g_{7/2}]_\nu + 10.3[3p_{3/2}2d_{5/2}]_\nu$ | 152 | 96 | 56 | 0.80 | 56.0 | 44.0 |
| $^{94}$Mo | 17.52$^*$ | $25.2[1f_{7/2}2d_{5/2}]_\pi + 18.9[1f_{5/2}1g_{7/2}]_\pi + 10.8[1g_{9/2}1h_{11/2}]_\nu + 10.1[1f_{7/2}1g_{9/2}]_\pi$ | 190 | 102 | 88 | | 31.4 | 68.6 |
| $^{96}$Mo | 10.36 | $34.8[2p_{1/2}3s_{1/2}]_\pi + 30.3[2p_{1/2}3s_{1/2}]_\nu + 14.4[2p_{3/2}2d_{5/2}]_\pi + 13.0[2f_{7/2}2d_{5/2}]_\nu$ | 132 | 82 | 50 | 0.72 | 48.6 | 51.4 |
| $^{96}$Mo | 11.33 | $24.3[2f_{7/2}2d_{5/2}]_\nu + 23.8[2d_{5/2}1f_{5/2}]_\pi + 17.6[2p_{3/2}2d_{5/2}]_\pi$ | 138 | 94 | 44 | 0.75 | 43.8 | 56.2 |
| $^{96}$Mo | 11.96 | $19.5[1f_{5/2}1g_{7/2}]_\pi + 13.9[1f_{5/2}1g_{7/2}]_\nu + 11.9[2d_{3/2}2p_{1/2}]_\pi$ | 172 | 106 | 66 | 0.93 | 45.4 | 54.6 |
| $^{96}$Mo | 12.46 | $57.7[1g_{7/2}2f_{7/2}]_\nu + 14.2[2d_{5/2}3p_{3/2}]_\nu$ | 128 | 90 | 38 | 0.70 | 92.9 | 7.1 |
| $^{96}$Mo | 12.47 | $60.2[1f_{5/2}2d_{5/2}]_\nu + 28.5[2d_{5/2}3p_{3/2}]_\nu$ | 104 | 68 | 36 | 0.57 | 96.5 | 3.5 |
| $^{96}$Mo | 12.57 | $37.5[1g_{7/2}2f_{7/2}]_\nu + 17.2[2d_{5/2}3p_{3/2}]_\nu + 12.5[1f_{5/2}2d_{5/2}]_\nu$ | 114 | 80 | 34 | 0.62 | 91.5 | 8.5 |
| $^{96}$Mo | 14.49 | $28.1[2p_{3/2}2d_{3/2}]_\pi + 18.2[1f_{5/2}2d_{3/2}]_\pi + 13.9[1g_{7/2}2f_{5/2}]_\nu$ | 144 | 108 | 36 | 0.78 | 41.7 | 58.3 |
| $^{96}$Mo | 13.54$^\dagger$ | $15.9[3p_{1/2}3s_{1/2}]_\nu + 13.8[2f_{5/2}2d_{5/2}]_\nu + 12.0[1f_{5/2}1g_{7/2}]_\nu$ | 158 | 100 | 58 | 0.86 | 74.5 | 25.6 |
| $^{96}$Mo | 17.50$^*$ | $53.7[1f_{7/2}2d_{5/2}]_\nu + 14.1[1f_{5/2}1g_{7/2}]_\nu$ | 184 | 104 | 80 | | 83.3 | 16.8 |
| $^{98}$Mo | 11.33 | $25.4[1f_{5/2}2d_{5/2}]_\pi + 22.0[2d_{5/2}2f_{7/2}]_\nu + 10.8[2p_{3/2}2d_{5/2}]_\pi$ | 160 | 104 | 56 | 0.81 | 40.0 | 60.0 |
| $^{98}$Mo | 12.45 | $49.7[2d_{5/2}3p_{3/2}]_\nu + 17.1[2p_{1/2}2d_{3/2}]_\pi$ | 134 | 92 | 42 | 0.68 | 76.9 | 23.1 |
| $^{98}$Mo | 14.53 | $38.7[2p_{3/2}2d_{3/2}]_\pi + 15.7[1f_{5/2}2d_{3/2}]_\pi + 12.2[2p_{3/2}3s_{1/2}]_\pi$ | 130 | 90 | 40 | 0.66 | 29.6 | 70.4 |
| $^{98}$Mo | 13.78$^\dagger$ | $18.1[2f_{5/2}2d_{5/2}]_\nu + 17.5[2p_{3/2}2d_{3/2}]_\pi + 15.5[2d_{3/2}3p_{1/2}]_\nu$ | 148 | 94 | 54 | 0.75 | 64.3 | 35.7 |
| $^{98}$Mo | 17.19$^*$ | $36.7[1f_{7/2}2d_{5/2}]_\pi + 18.3[1f_{5/2}1g_{7/2}]_\pi$ | 198 | 104 | 94 | | 22.3 | 77.8 |
